# Supplementary material for: Defects Enhance Stability in 12-fold Symmetric Soft-Matter Quasicrystals
Source: arXiv:2408.08168 ancillary file (2025-06-12)
Supplement: Supplementary file 1 [file SM.pdf]

# Supplemental Material: Defects Enhance Stability in 12-fold Symmetric Soft-Matter Quasicrystals

Alptuğ Ulugöl,<sup>1,\*</sup> Robert J. Hardeman,<sup>1</sup> Frank Smalenburg,<sup>2</sup> and Laura Filion<sup>1</sup>

<sup>1</sup>*Soft Condensed Matter and Biophysics, Debye Institute of Nanomaterials Science, Utrecht University, Utrecht, Netherlands*

<sup>2</sup>*Université Paris-Saclay, CNRS, Laboratoire de Physique des Solides, 91405 Orsay, France*

(Dated: January 17, 2025)

## CONTENTS

|                                                                                    |   |
|------------------------------------------------------------------------------------|---|
| I. Constraints on the distribution of tiles                                        | 1 |
| A. Constraint 1: Simply-connected tiling                                           | 1 |
| B. Constraint 2: Global uniformity                                                 | 1 |
| C. Constraint 3: Rotational symmetry                                               | 2 |
| II. Methodological Details                                                         | 3 |
| A. Open Boundaries and Tile Biasing                                                | 3 |
| B. Markov-Chain Monte Carlo Simulation                                             | 3 |
| 1. Vertex Moves                                                                    | 3 |
| 2. Swap Moves                                                                      | 4 |
| C. Configurational Entropy Calculation                                             | 5 |
| III. 2D Structure Factors of Single Snapshots                                      | 7 |
| IV. Alternative Representation of the Plots from Figure 2 a & c from the Main Text | 7 |
| V. Mapping Rhombi into Shields and Eggs                                            | 7 |
| References                                                                         | 9 |

## I. CONSTRAINTS ON THE DISTRIBUTION OF TILES

Here, we investigate the theoretical constraints on the tile compositions of 12-fold symmetric square-triangle-rhombus tilings in the thermodynamic limit. To this end, we follow the approach of Refs. [1–3]. We consider a large patch of tiling, consisting entirely of squares, equilateral triangles, and rhombi, all with identical edge lengths. Such a tiling can be described by its area fractions of squares, triangles, and rhombi of different orientations. In particular, we denote the total area fractions of each type of tile as

$$\sigma = \sum_{i=1}^3 \sigma_i, \quad \tau = \sum_{i=1}^4 \tau_i, \quad \rho = \sum_{i=1}^6 \rho_i, \quad (\text{S1})$$

with the subscripted area fractions  $\sigma_i$ ,  $\tau_i$ , and  $\rho_i$  denoting the fraction of patch area covered by squares, triangles, and rhombi of orientation  $i$ , respectively. We denote a square of orientation  $i$  as an  $S_i$  square, and similarly  $T_i$

and  $R_i$  for triangles, and rhombi. Illustrations of each of the tile orientations can be seen in Table S1. In total, this corresponds to 13 degrees of freedom. In the following, we derive constraints on this set of parameters in order to make predictions about the tile concentrations for general random square-triangle-rhombus tilings.

### A. Constraint 1: Simply-connected tiling

The first assumption we make about our tiling is that it is free of holes and overlaps. In other words, there are no tile shapes other than squares, triangles, or rhombi, and that all space enclosed by the perimeter of the tiling is covered by exactly one tile. This leads to our first constraint on the tile concentration:

$$\sigma + \tau + \rho = 1, \quad (\text{S2})$$

which simply states that all of space must be covered by tiles.

### B. Constraint 2: Global uniformity

The second assumption we make about our patch of tiling is that it is globally uniform: if we take a large enough sub-patch of the tiling, it should have approximately the same tile concentrations as the overall patch, regardless of the location of the sub-patch.

As shown in Ref. [1], the global uniformity condition gives rise to the following constraint:

$$\det \langle B \rangle = \langle \det B \rangle, \quad (\text{S3})$$

where  $B$  is the hyperslope of the mapping from the parallel-space to the perpendicular-space representation of the tiling. The hyperslopes of the individual tiles are given in Table S1 (see also Ref. [3]).

For the square-triangle-rhombus tilings, the average hyperslope-determinant is given by

$$\begin{aligned} \langle \det B \rangle &= \sum_{i=1}^3 \sigma_i \det B_{S_i} + \sum_{i=1}^4 \tau_i \det B_{T_i} + \sum_{i=1}^6 \rho_i \det B_{R_i} \\ &= - \sum_{i=1}^3 \sigma_i + \sum_{i=1}^4 \tau_i - \sum_{i=1}^6 \rho_i \\ &= \tau - (\sigma + \rho). \end{aligned} \quad (\text{S4})$$

\* a.ulugol@uu.nl

Similarly, the determinant of the average hyperslope is given by

$$\begin{aligned} \det \langle B \rangle = & 12(\rho_1\rho_3 - \rho_1\rho_4 + \rho_1\rho_5 + \rho_2\rho_4 \\ & - \rho_2\rho_5 + \rho_2\rho_6 + \rho_4\rho_6 + \rho_3\rho_5 - \rho_3\rho_6) \\ & + 6(\rho_1\sigma_3 + \rho_2\sigma_1 + \rho_3\sigma_2 + \rho_4\sigma_3 + \rho_5\sigma_1 + \rho_6\sigma_2) \\ & - 4(\tau_1\tau_2 + \tau_2\tau_3 + \tau_3\tau_4 + \tau_4\tau_1) \\ & + 3(\sigma_1\sigma_2 + \sigma_2\sigma_3 + \sigma_3\sigma_1) \\ & + \tau^2 - (\sigma + \rho)^2. \end{aligned} \quad (\text{S5})$$

### C. Constraint 3: Rotational symmetry

Finally, in order to restrict ourselves to quasicrystalline tilings with 12-fold symmetry, we impose that for each tile, all orientations occur equally frequently:

$$\sigma_i = \frac{\sigma}{4}, \quad \tau_i = \frac{\tau}{3}, \quad \rho_i = \frac{\rho}{6}. \quad (\text{S6})$$

As a result of this, the right-hand side of Eq. S5 vanishes, and hence Eq. S3 reduces to:

$$\tau - (\sigma + \rho) = 0. \quad (\text{S7})$$

Finally, combining equations (S2) and (S7) yields the theoretical constraints on the area fractions [3]:

$$\tau = \frac{1}{2}, \quad \sigma + \rho = \frac{1}{2}. \quad (\text{S8})$$

| $X_i$ | Tile                                                                                | Area                    | $B_{X_i}$                                                               | $\det B_{X_i}$ |
|-------|-------------------------------------------------------------------------------------|-------------------------|-------------------------------------------------------------------------|----------------|
| $S_1$ | 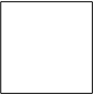 | $a^2$                   | $\begin{pmatrix} 1 & 0 \\ 0 & -1 \end{pmatrix}$                         | -1             |
| $S_2$ | 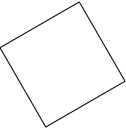 | $a^2$                   | $\begin{pmatrix} -1/2 & -\sqrt{3}/2 \\ -\sqrt{3}/2 & 1/2 \end{pmatrix}$ | -1             |
| $S_3$ | 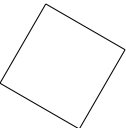 | $a^2$                   | $\begin{pmatrix} -1/2 & \sqrt{3}/2 \\ \sqrt{3}/2 & 1/2 \end{pmatrix}$   | -1             |
| $T_1$ | 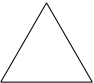 | $\frac{\sqrt{3}}{4}a^2$ | $\begin{pmatrix} 1 & 0 \\ 0 & 1 \end{pmatrix}$                          | 1              |

|       |                                                                                      |                         |                                                                |    |
|-------|--------------------------------------------------------------------------------------|-------------------------|----------------------------------------------------------------|----|
| $T_2$ | 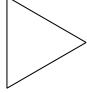   | $\frac{\sqrt{3}}{4}a^2$ | $\begin{pmatrix} -1 & 0 \\ 0 & -1 \end{pmatrix}$               | 1  |
| $T_3$ | 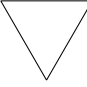   | $\frac{\sqrt{3}}{4}a^2$ | $\begin{pmatrix} 1 & 0 \\ 0 & 1 \end{pmatrix}$                 | 1  |
| $T_4$ | 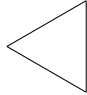   | $\frac{\sqrt{3}}{4}a^2$ | $\begin{pmatrix} -1 & 0 \\ 0 & -1 \end{pmatrix}$               | 1  |
| $R_1$ | 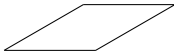   | $\frac{1}{2}a^2$        | $\begin{pmatrix} 1 & -2\sqrt{3} \\ 0 & -1 \end{pmatrix}$       | -1 |
| $R_2$ | 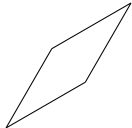  | $\frac{1}{2}a^2$        | $\begin{pmatrix} -2 & \sqrt{3} \\ -\sqrt{3} & 2 \end{pmatrix}$ | -1 |
| $R_3$ | 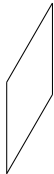 | $\frac{1}{2}a^2$        | $\begin{pmatrix} 1 & 0 \\ 2\sqrt{3} & -1 \end{pmatrix}$        | -1 |
| $R_4$ | 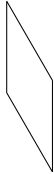 | $\frac{1}{2}a^2$        | $\begin{pmatrix} 1 & 0 \\ -2\sqrt{3} & -1 \end{pmatrix}$       | -1 |
| $R_5$ | 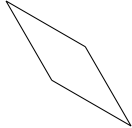 | $\frac{1}{2}a^2$        | $\begin{pmatrix} -2 & -\sqrt{3} \\ \sqrt{3} & 2 \end{pmatrix}$ | -1 |
| $R_6$ | 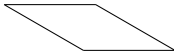 | $\frac{1}{2}a^2$        | $\begin{pmatrix} 1 & 2\sqrt{3} \\ 0 & -1 \end{pmatrix}$        | -1 |

TABLE S1: The properties of the different tile orientations encountered in a square-triangle-rhombus tiling. The areas are given for edges of length  $a$ . The hyperslopes are the Jacobian matrices of the mapping of vertices between parallel and perpendicular space.

## II. METHODOLOGICAL DETAILS

In this section we introduce the details of the open boundary simulations and describe the analysis methods for the square-triangle-rhombus tilings. We start by describing our model, in particular, how the open boundaries and tile biasing are introduced. Then, we describe how the initial square-triangle tiling is generated. Next, we introduce the vertex and swap moves for the Monte Carlo simulation. Finally, we explain how the simulation data is analysed, i.e., how the unbiasing and thermodynamic integration is performed to obtain the configurational entropy of square-triangle-rhombus tiling.

### A. Open Boundaries and Tile Biasing

Putting quasicrystals into a periodic simulation box necessarily breaks the inherent aperiodicity of the quasicrystal, making it difficult to unravel in simulations whether defects appear due to kinetic trapping or their influence on the free energy of the system. In an effort to address this, we introduce a new simulation method designed to explore square-triangle-rhombus tilings under open boundary conditions by incorporating a confining line tension, denoted by  $\gamma$ . Specifically, in our simulations we consider a single patch of square-triangle-rhombus tiling on a quasicrystalline lattice, and include a boundary contribution to the potential energy, given by

$$U_B = \gamma L, \quad (\text{S9})$$

where  $L$  denotes the circumference of the tiling. This contribution biases the system towards compact configurations while letting the tiling evolve to most favorable boundary shape for a given value of  $\gamma$ . Note that in the thermodynamic limit ( $N \rightarrow \infty$ ), the effects of the boundary are expected to vanish and hence in this limit our results should become independent of our choice of  $\gamma$ .

To control the tile composition of the system, we introduce a chemical potential-like energy contribution for every tile type,

$$U_{\mathcal{T}} = \sum_{t \in \mathcal{T}} \epsilon_t n_t, \quad (\text{S10})$$

where  $\epsilon_t$ ,  $n_t$  are the energy contribution and the number of tile type  $t$ . The set of tile types is defined as  $\mathcal{T} = \{S, T, R\}$  representing squares, triangles and rhombi

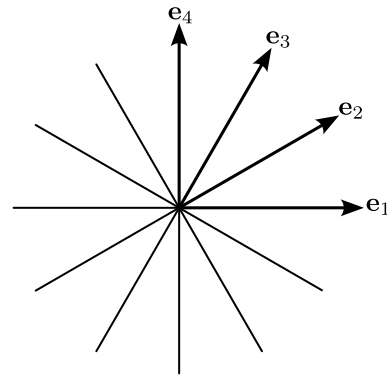

FIG. S1. Possible connected neighbor positions of a vertex.

respectively. Using this biasing potential, we can explore the free energies of different tile compositions by changing the energy contribution of each tile type. For the purpose of this paper we focus on systems where  $\epsilon_S = \epsilon_T = 0$ , and hence only vary  $\epsilon_R$ .

With both energy contributions, Eqs.(S9,S10), combined, we arrive at the total energy that we use to simulate the system,

$$U = U_B + U_{\mathcal{T}} = \gamma L + \epsilon_R n_R. \quad (\text{S11})$$

Having established the model, we proceed with the introduction of the simulation details.

### B. Markov-Chain Monte Carlo Simulation

Here we consider Markov Chain Monte Carlo (MCMC) simulations of tilings with a fixed number of vertices and let the number of squares, triangles, and rhombi fluctuate. We use two types of MC moves: (i) vertex moves and (ii) swap moves. The vertex moves enable local rearrangements of the tiling and the swap moves enable non-local transport of vertices. We provide the details of these moves in the following.

#### 1. Vertex Moves

To construct a vertex move, first, we need to identify every possible position a vertex can have with respect to its neighbours. When we consider every orientation of the allowed tiles, we find that the relative position of two connected vertices can assume twelve possible vectors as shown in Figure (S1) where every subsequent vector is a  $\pi/6$  rotation of the previous. Therefore we perform our simulation on a quasicrystalline lattice where each potential vertex location is connected to 12 others. One way to construct a vertex move is to choose a pair of existing connected vertices and rotate one of the vertices

around the other by an angle of  $\pi/6$  clockwise or counter-clockwise. This type of vertex move enables tile propagation in the bulk and tile creation/annihilation at the boundary. However, this move should be implemented with care to allow only square, triangle, and rhombus tiles to exist and obey detailed balance. Our implementation of the vertex move consists of eight steps:

1. Choose a random vertex,  $i$ , in the tiling to displace.
2. Choose a random direction out of the 12 possible directions that a connected neighbor of vertex  $i$  could occupy.
3. If there is a vertex in the randomly chosen direction, identify it as the vertex  $j$ . Otherwise reject the move. Vertex  $j$  is the pivot of vertex  $i$ 's rotation.
4. Choose a random rotation direction, i.e., clockwise or counter-clockwise. Rotate vertex  $i$  around vertex  $j$  by  $\pi/6$  in the chosen direction.
5. If vertex  $i$  overlaps with another vertex, reject the move.
6. Check the tiles which are altered by vertex  $i$ 's movement. If there is an invalid tile, i.e., a tile which is not a square, a triangle or a rhombus, reject the move. An example is depicted in Figure (S2)
7. Check if the tiling remains connected. If the tiling separated into multiple disconnected pieces, reject the move.
8. Accept the move with probability,

$$P_{\text{acc}}(i \rightarrow f) = \min \left( 1, e^{-\beta(U_f - U_i)} \right), \quad (\text{S12})$$

where  $U_{i,f}$  are the potential energies of the initial and final state given by Eq. (S11). Note that  $\beta = 1/k_B T$  is the inverse thermal energy.

Since this implementation of the vertex moves propagates the tiles in the bulk without changing the tile counts or the boundary length, valid bulk moves are always accepted. A sample vertex move in bulk is depicted in Figure S3(a). Moreover, the fluctuations on the boundary facilitate the creation and the annihilation of different tiles. Therefore, the dynamics of the MCMC algorithm can be summarized by (i) tile creation/annihilation at the boundary and (ii) propagation of tiles in the bulk. However, due to many validation steps in the algorithm, the majority of the proposed moves end up being invalid, resulting in relatively low acceptance rates.

## 2. Swap Moves

To improve the equilibration times we propose another type of move which we call a swap move. To construct

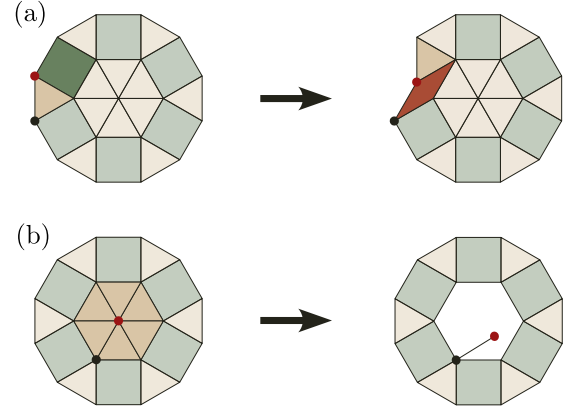

FIG. S2. The red vertex attempts to rotate clockwise around the blue vertex by an angle of  $\pi/6$ . (a) The move results in a valid tiling and may be accepted. (b) The move results in an invalid tiling and is rejected.

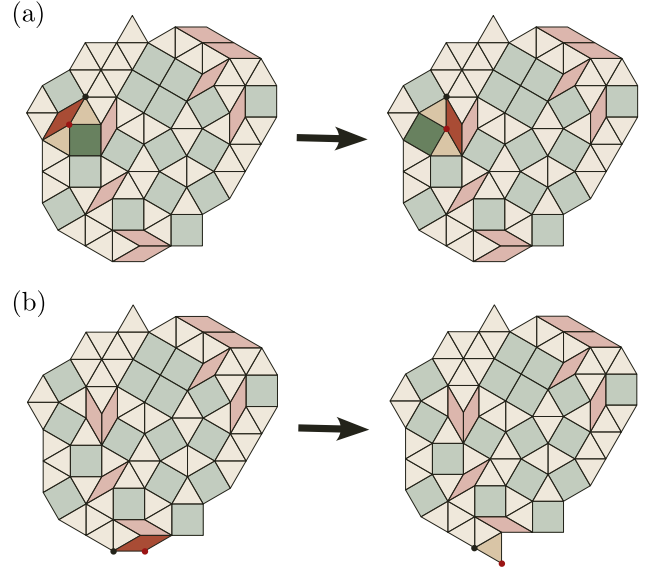

FIG. S3. Sample vertex moves in (a) bulk and at (b) the boundary.

this move, we focus on the pentagonal patches in the square-triangle-rhombus tiling. In our system there is only one allowed pentagonal patch, whose internal angles are  $(\pi/3, 5\pi/6, \pi/2, \pi/2, 5\pi/6)$ . As shown in Figure (S4), this pentagonal region has two different decompositions: (i) it can be decomposed into a square and a triangle, which we call the “house” configuration or (ii) it can be decomposed into two rhombi and a triangle, which we refer as the “ $R^2T$ ” configuration.

After we identify these patches in the tiling, we perform the move by swapping a random pair of disjoint house and  $R^2T$  patches as seen in Fig(S5). Therefore, we implement the swap moves in three steps as:

1. Identify all house configurations in the tiling and randomly choose one.

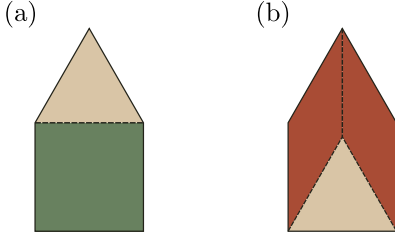

FIG. S4. The decompositions of the pentagonal patch: (a) the house configuration and (b) the  $R^2T$  configuration.

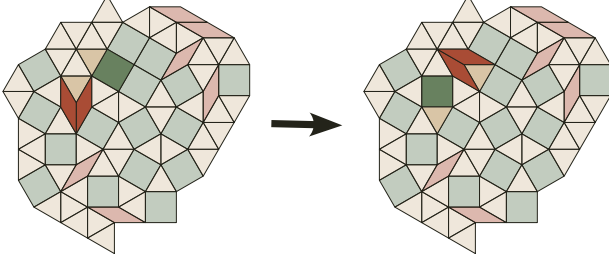

FIG. S5. An example of the swap move.

2. Identify all  $R^2T$  configurations in the tiling and randomly choose one.
3. If the chosen house and  $R^2T$  configurations are not disjoint, reject the move. Otherwise, accept the move and swap the configurations.

As the number of house and  $R^2T$  configurations do not change with swap moves, detailed balance is trivially satisfied. Moreover, since the swap moves do not change either the tile counts or the boundary length, they do not cause a potential energy change and are always accepted if they are valid. This results in a high acceptance rate. The non-local nature of the swap moves enables rapid rhombi propagation from boundary to bulk. This promotes local bulk rearrangements via vertex moves and speeds up the equilibration process.

In the following subsection, we explain how we use the simulation results to calculate the configurational entropy of the square-triangle-rhombus tiling.

### C. Configurational Entropy Calculation

To calculate the configurational entropy of the square-triangle-rhombus tiling, we first calculate the free energy of the tiling using thermodynamic integration with the pure square-triangle tiling as the reference state. Thus, the free energy of the square-triangle-rhombus tiling is given by

$$F(N, \gamma, T; \epsilon_R) = F_{\text{sq-tr}}(N, \gamma, T) - \Delta F(N, \gamma, T; \epsilon_R) \quad (\text{S13})$$

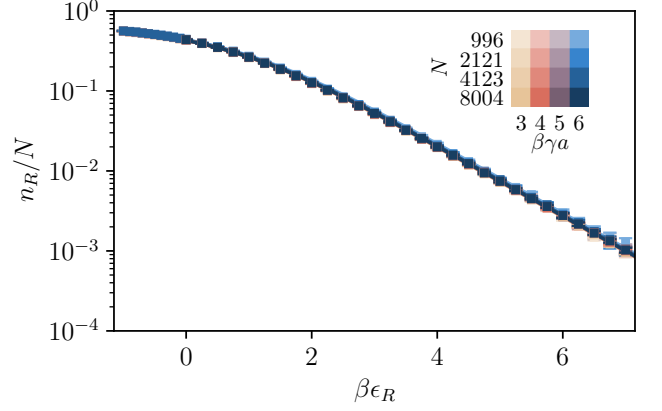

FIG. S6. The ensemble average of the number of rhombi with respect to varying rhombi biasing potential.

where the free energy difference  $\Delta F(N, \gamma, T; \epsilon_R)$  is

$$\begin{aligned} \Delta F(N, \gamma, T; \epsilon_R) &= \int_{\epsilon_R}^{\infty} d\epsilon'_R \frac{dF(N, \gamma, T; \epsilon_R)}{d\epsilon_R}, \\ &= \int_{\epsilon_R}^{\infty} d\epsilon'_R \left\langle \frac{dU}{d\epsilon_R} \right\rangle_{N, \gamma, T, \epsilon'_R}, \quad (\text{S14}) \\ &= k_B T \int_{\epsilon_R}^{\infty} d\epsilon'_R \langle n_R \rangle_{N, \gamma, T, \epsilon'_R}, \end{aligned}$$

where  $\langle \dots \rangle$  represents an ensemble average. The free energy difference depends on the ensemble average of the number of rhombi,  $\langle n_R \rangle_{N, \gamma, T, \epsilon'_R}$ , in the tiling. Therefore, we need the functional form of this quantity to perform the thermodynamic integration.

The family of the functions that can describe the number of rhombi has three physical constraints that we need to impose: number of rhombi has to (i) decrease monotonically with increasing  $\epsilon_R$ , (ii) approach  $N$  when  $\epsilon_R \rightarrow -\infty$ , and (iii) decay to 0 exponentially when as  $\epsilon_R \rightarrow \infty$ . When we impose these constraints and inspect our simulation results shown in Figure (S6), we see that the number of rhombi is well fitted by the function given by

$$\frac{\langle n_R \rangle_{N, \gamma, T, \epsilon_R}}{N} = \frac{1 + \nu_R e^{-\beta(\epsilon_R - \mu_R)/2}}{e^{\beta(\epsilon_R - \mu_R)} + \nu_R e^{-\beta(\epsilon_R - \mu_R)/2} + 2} \quad (\text{S15})$$

where  $\mu_R$  is the offset energy, and  $\nu_R > 0$  is the shape parameter. Here, we observe the offset energy, and the shape parameter are parameters that depend on the system size and line tension listed in Table S2.

Then, we can obtain the closed form expression for the free energy difference by plugging Eq.(S15) into Eq.(S14)

| $N$  | $\beta\gamma a$ | $\beta\mu_R$ | $\nu_R$ | $\beta\mu_\rho$ | $\nu_\rho$ | $\beta\mu_L$ | $\nu_L$ | $L_\infty/Na$ | $\omega$ |
|------|-----------------|--------------|---------|-----------------|------------|--------------|---------|---------------|----------|
| 996  | 3               | 0.06         | 0.42    | -0.46           | 0.23       | 1.80         | 0.18    | 0.13          | 1.39     |
| 996  | 4               | 0.08         | 0.42    | -0.44           | 0.23       | 1.68         | 0.20    | 0.12          | 1.39     |
| 996  | 5               | 0.11         | 0.42    | -0.42           | 0.22       | 1.49         | 0.25    | 0.12          | 1.27     |
| 996  | 6               | 0.16         | 0.40    | -0.36           | 0.20       | 1.32         | 0.31    | 0.12          | 1.17     |
| 2121 | 3               | 0.06         | 0.44    | -0.48           | 0.23       | 1.96         | 0.13    | 0.09          | 1.72     |
| 2121 | 4               | 0.08         | 0.43    | -0.47           | 0.22       | 1.70         | 0.19    | 0.08          | 1.41     |
| 2121 | 5               | 0.09         | 0.43    | -0.45           | 0.21       | 1.47         | 0.23    | 0.08          | 1.33     |
| 2121 | 6               | 0.11         | 0.44    | -0.44           | 0.22       | 0.86         | 0.42    | 0.08          | 0.97     |
| 4123 | 3               | 0.06         | 0.45    | -0.49           | 0.21       | 1.67         | 0.20    | 0.07          | 1.26     |
| 4123 | 4               | 0.07         | 0.44    | -0.49           | 0.21       | 1.63         | 0.19    | 0.06          | 1.34     |
| 4123 | 5               | 0.08         | 0.44    | -0.47           | 0.20       | 1.33         | 0.26    | 0.06          | 1.17     |
| 4123 | 6               | 0.11         | 0.43    | -0.45           | 0.19       | 0.69         | 0.43    | 0.06          | 0.97     |
| 8004 | 3               | 0.05         | 0.46    | -0.52           | 0.26       | 1.74         | 0.18    | 0.05          | 1.29     |
| 8004 | 4               | 0.07         | 0.43    | -0.51           | 0.23       | 1.17         | 0.28    | 0.04          | 1.13     |
| 8004 | 5               | 0.07         | 0.43    | -0.50           | 0.22       | 1.10         | 0.32    | 0.04          | 1.12     |
| 8004 | 6               | 0.08         | 0.42    | -0.49           | 0.22       | 1.69         | 0.18    | 0.04          | 1.46     |

TABLE S2. Fit parameters of Eqs.(S15, S19, S20) for the simulation data at different system sizes and line tensions.

and performing the integral. This yields,

$$\Delta F(N, \gamma, T; \epsilon_R) = -2Nk_B T \left[ \sum_{k=1}^3 \frac{(1 + \nu_R z_k) \log(-z_k)}{4 + 3\nu_R z_k} - \sum_{k=1}^3 \frac{(1 + \nu_R z_k) \log(e^{-\beta(\epsilon_R - \mu_R)/2} - z_k)}{4 + 3\nu_R z_k} \right], \quad (\text{S16})$$

where  $z_k$  are the three solutions of the following cubic equation,

$$\nu_R z_k^3 + 2z_k^2 + 1 = 0.$$

To calculate the entropy, we recall the fundamental identity,  $F = U - TS$ , relating the energy and the entropy to the free energy. Then, we can rewrite the free energy difference  $\Delta F(N, \gamma, T; \epsilon_R)$  as

$$\begin{aligned} \Delta F(N, \gamma, T; \epsilon_R) &= \Delta U(N, \gamma, T; \epsilon_R) - T\Delta S(N; \epsilon_R), \\ &= \epsilon_R n_R(N, \gamma, T; \epsilon_R) \\ &\quad + \gamma [L(N, \gamma, T; \infty) - L(N, \gamma, T; \epsilon_R)] \\ &\quad - T[S_{\text{sq-tr}} - S(N; \epsilon_R)], \end{aligned} \quad (\text{S17})$$

where in the first line of the second step, we used  $\epsilon_R n_R \rightarrow 0$  as  $\epsilon_R \rightarrow \infty$ . Furthermore, the configurational entropy of the square-triangle tiling per vertex is exactly calculated in the literature [4, 5] using Bethe ansatz to be

$$\frac{S_{\text{sq-tr}}}{Nk_B} = \log(108) - 2\sqrt{3} \log(2 + \sqrt{3}) = 0.12005524 \dots$$

Then, we can rearrange Eq.(S17) to obtain the configurational entropy of the square-triangle-rhombus tiling as

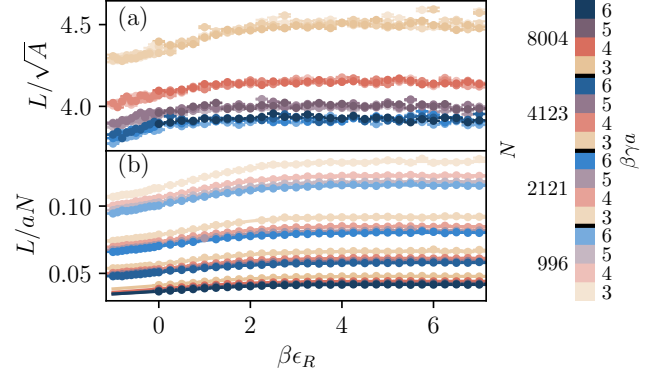

FIG. S7. The ensemble average of the boundary length with respect to varying rhombi biasing potential.

a function of the measurable quantities as

$$\begin{aligned} \frac{S(N; \epsilon_R)}{Nk_B} &= \frac{S_{\text{sq-tr}}}{Nk_B} + \frac{\beta\epsilon_R}{N} \langle n_R \rangle_{N, \gamma, T, \epsilon_R} \\ &\quad + \frac{\beta\gamma}{N} [\langle L \rangle_{N, \gamma, T, \epsilon_R} - \langle L \rangle_{N, \gamma, T, \infty}] \\ &\quad - \frac{1}{N} \beta \Delta F(N, \gamma, T; \epsilon_R), \end{aligned} \quad (\text{S18})$$

where  $\langle n_R \rangle_{N, \gamma, T, \epsilon_R}$  and  $\Delta F(N, \gamma, T; \epsilon_R)$  are given by Eq. (S15) and Eq. (S16) respectively. To calculate the configurational entropy from our simulations, we still need a function describing the behavior of the boundary length,  $\langle L \rangle_{N, \gamma, T, \epsilon_R}$ . Similar to the number of rhombi, the boundary length is also bounded from above and below. In particular, the bounds are given by

$$\sqrt{2\pi N} < L/a \leq 2N - 2,$$

where  $a$  is the tile edge length, the lower and the upper bounds are the circular rhombus tiling and linear chain limits, respectively. Upon inspection of our simulation data as seen in Figure S7, we observe that the boundary length follows a generalized logistic function given by

$$\langle L \rangle_{N, \gamma, T, \epsilon_R} = \sqrt{2\pi N} + \frac{L_\infty - \sqrt{2\pi N}}{(1 + e^{-\omega\beta(\epsilon_R - \mu_L)})^{\nu_L}}, \quad (\text{S19})$$

where  $L_\infty$  is the boundary length at the square-triangle tiling limit,  $\mu_L$  is the offset energy,  $\nu_L > 0$  is the shape parameter, and  $\omega > 0$  is the tail parameter. Similar to the number of rhombi, we observe that the fit parameters depend on the system size and line tension as listed in Table S2. Then, when we plug Eqs.(S15, S16, S19) into Eq.(S18), we get the configurational entropy per vertex parameterized by the rhombus biasing potential  $\epsilon_R$ . Moreover, the size dependence,  $N$ , drops out in the infinite system limit since entropy per vertex is an intensive variable. Thus, we define the configurational entropy per vertex as

$$s(\epsilon_R) = \frac{S(N; \epsilon_R)}{N}.$$

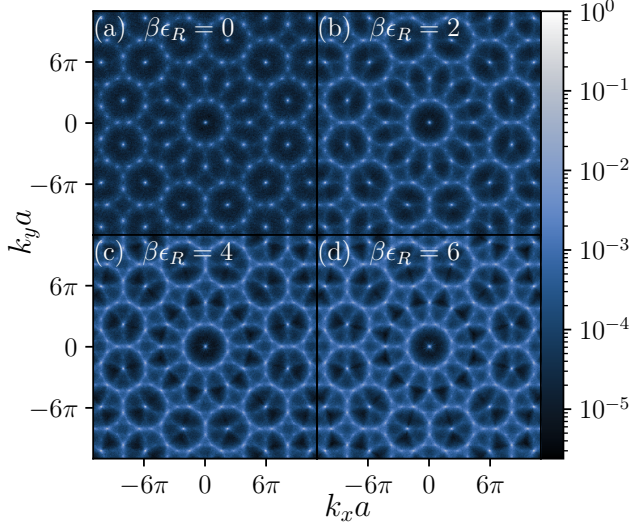

FIG. S8. 2D structure factors of single snapshots of the tilings at  $N = 8004$ ,  $\beta\gamma a = 4$ ,  $\beta\epsilon_R =$  (a) 0, (b) 2, (c) 4, and (d) 6. The structure factors are Gaussian blurred with standard deviation  $0.07/a$  to increase visibility.

Finally, we parameterize the area fraction of rhombi similar to  $n_R$  as

$$\langle \rho \rangle_{N,\gamma,T,\epsilon_R} = \frac{1 + \nu_\rho e^{-\beta(\epsilon_R - \mu_\rho)/2}}{e^{\beta(\epsilon_R - \mu_\rho)} + \nu_\rho e^{-\beta(\epsilon_R - \mu_\rho)/2} + 2}, \quad (\text{S20})$$

where the fit parameters are listed in Table S2. Then the configurational entropy per vertex,  $s(\rho)$ , is fully characterized by Eq.(S18) and Eq.(S20).

### III. 2D STRUCTURE FACTORS OF SINGLE SNAPSHOTS

Here we show that the 2D structure factors of single snapshots of the tiling remains consistent with 12-fold symmetry as seen in Fig S8.

### IV. ALTERNATIVE REPRESENTATION OF THE PLOTS FROM FIGURE 2 A & C FROM THE MAIN TEXT

Due to the overlap of the curves in Fig. 2(a,c), we present them in an alternative way in Fig. S9 and Fig. S10 to improve clarity. Specifically, using  $N_{\text{ref}} = 4123$ ,  $\beta\gamma_{\text{ref}}a = 4$  as a reference point, we define the relative configurational entropy as  $\delta S(N, \gamma, \epsilon_R) := S(N, \gamma, \epsilon_R) - S(N_{\text{ref}}, \gamma_{\text{ref}}, \epsilon_R)$ . The corresponding relative configurational entropies are then plotted against the rhombus biasing potential ( $\epsilon_R$ ) and the rhombus area fraction ( $\rho$ ).

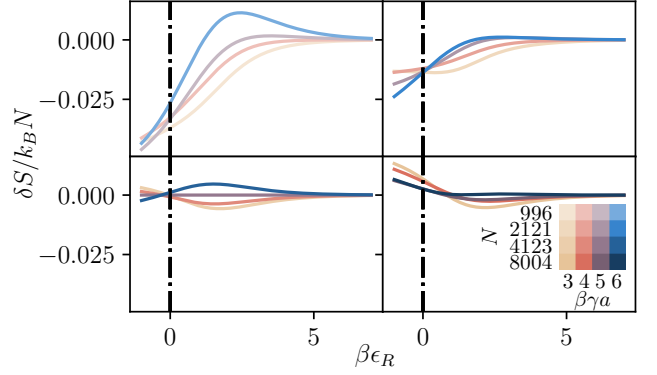

FIG. S9. Relative configurational entropy per vertex as a function of the rhombus biasing potential. Shown is the difference with respect to a reference system with  $N_{\text{ref}} = 4123$ ,  $\beta\gamma_{\text{ref}}a = 4$ .

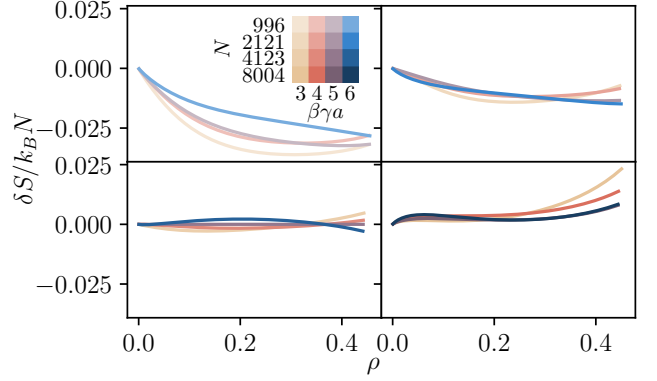

FIG. S10. Relative configurational entropy per vertex as a function of the rhombus area fraction. Shown is the difference with respect to a reference system with  $N_{\text{ref}} = 4123$ ,  $\beta\gamma_{\text{ref}}a = 4$ .

### V. MAPPING RHOMBI INTO SHIELDS AND EGGS

Since shield and egg tiles can each be decomposed into a square, two triangles, and a rhombus, as shown in Fig. S11, we can construct a map between square-triangle-rhombus tilings and square-triangle-shield-egg tilings in the limit where rhombi are sufficiently far away from each other.

To understand the mapping, we analyze the entropy contributions of configurations with a single rhombus tile and their corresponding shield-egg tilings. This mapping provides insights into the relationship between the entropy of rhombus defects and that of shield/egg defects.

When we start with a configuration containing exactly one rhombus, it can be mapped into a square-triangle-shield-egg tiling in two distinct ways by choosing which obtuse-angled vertex to take out. From local neighborhood mapping results shown in Fig. S12, we observe that,

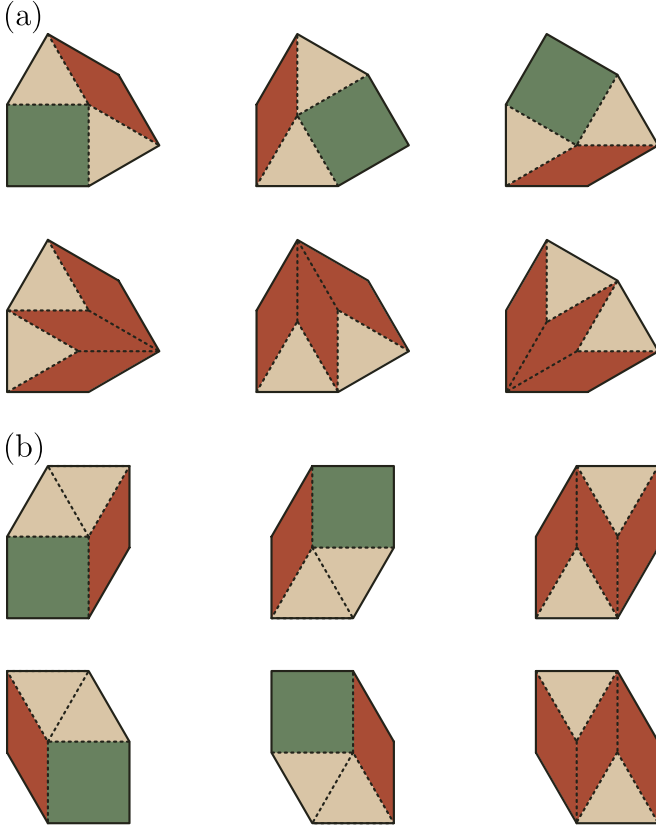

FIG. S11. Square-triangle-rhombus decorations of (a) the shield and (b) the egg tiles. In panel (b), the first row shows the decorations of left-handed egg and the second rows shows the right-handed egg.

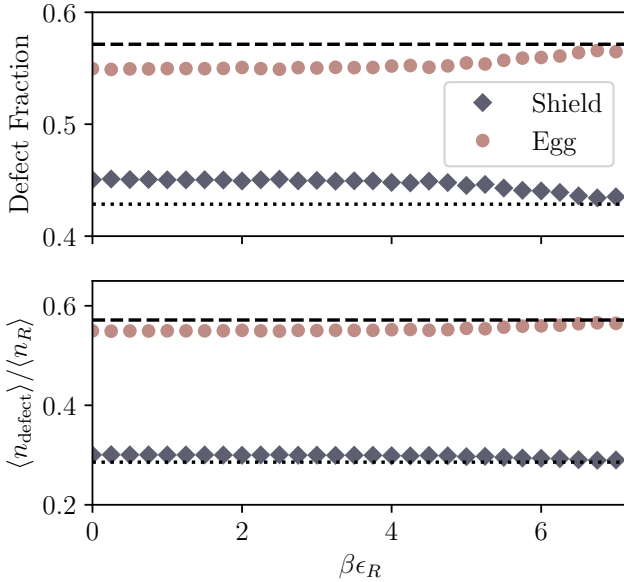

FIG. S12. Defect fraction and number of defects as a function of  $\beta\epsilon_R$  for shields, eggs defects mapped from rhombi. In the upper panel, dashed and dotted lines correspond to the values  $4/7$  and  $3/7$ , respectively. In the lower panel, dashed and dotted lines correspond to the values  $4/7$  and  $2/7$ , respectively.

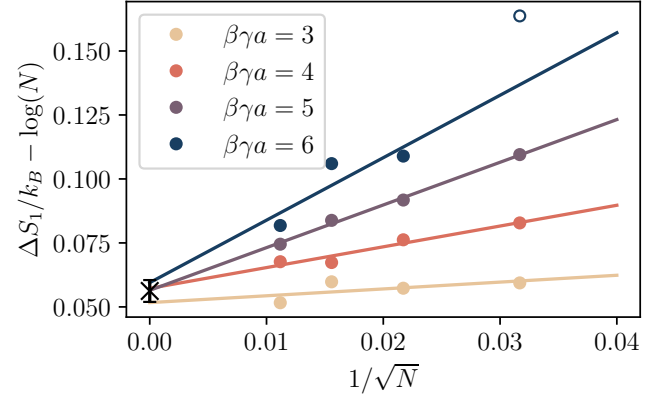

FIG. S13. Finite-size scaling of the configurational entropy difference,  $\Delta S_1/k_B - \log(N)$ , as a function of the inverse square root of number of vertices, for various line tensions  $\beta\gamma a$ . Linear fits demonstrate that the entropy converges to  $0.056(4)$  (the  $\times$  marker) in the thermodynamic limit ( $1/\sqrt{N} \rightarrow 0$ ).

in the limit of low rhombus concentrations, we can map the rhombi to shields and eggs with the probabilities  $3/7$  and  $4/7$ , respectively. However, due to the different decorations of the shield and egg tiles (i.e. the single-rhombus decorations shown in Fig. S11), shields are overcounted by a factor of 3, and eggs are overcounted by a factor of 2 in this mapping. To correct for this overcounting, we compute the number of distinct valid tilings that emerge from a single rhombus configuration.

For each rhombus, the average number of shield tiles generated is:

$$\frac{\langle n_{\text{Sh}} \rangle}{\langle n_R \rangle} = 2 \times \frac{1}{3} \times \frac{3}{7} = \frac{2}{7}$$

where the factors represent the choice of obtuse-angled vertex to take out, the overcounting-correction due to decorations and the mapping probability to a shield, respectively.

Similarly, the average number egg tiles is:

$$\frac{\langle n_{\text{Egg}} \rangle}{\langle n_R \rangle} = 2 \times \frac{1}{2} \times \frac{4}{7} = \frac{4}{7}$$

Thus, each tiling with a single rhombus generates an average of  $6/7$  tilings with either a shield or an egg, with eggs occurring twice as often as shields. This latter ratio can likely be attributed to the fact that egg tiles are chiral, and hence can occur in a left-handed or right-handed conformation, which cannot be mapped onto each other via rotation, as shown in Fig. S14(b). Hence, based on our measurements in Fig. S12, we predict that in the set of configurations with a single shield/egg defect, shields, left-handed eggs, and right-handed eggs all occur at the same frequency, and hence that these defect types have identical effects on the entropy of the tiling as long as they do not interact.

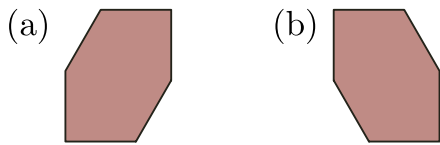

FIG. S14. Two chiralities of the egg tile: (a) left-handed egg, (b) right-handed egg.

As the transition from a rhombus to a shield or egg defect involved deleting a vertex, we finally have to replace the missing vertex. This placement contributes an

additional entropy of  $s_{\text{Sq-Tr}} \approx 0.12k_B$

Combining these factors, the entropy of a single shield/egg defect is related to the entropy of a single rhombus defect as follows:

$$\frac{\Delta S_{1,\text{Sh/Egg}}}{k_B} = \frac{\Delta S_{1,\text{R}}}{k_B} + \log\left(\frac{6}{7}\right) + \frac{s_{\text{Sq-Tr}}}{k_B} \approx 0.022 + \log N. \quad (\text{S21})$$

This is noticeably lower than the  $\Delta S_{1,\text{R}}/k_B \simeq 0.056 + \log N$  we found for a rhombus defect.

- 
- [1] M. Impérator-Clerc, A. Jagannathan, P. Kalugin, and J.-F. Sadoc, Square-triangle tilings: An infinite playground for soft matter, *Soft Matter* **17**, 9560 (2021).
  - [2] E. Fayen, M. Impérator-Clerc, L. Filion, G. Foffi, and F. Smalenburg, Self-assembly of dodecagonal and octagonal quasicrystals in hard spheres on a plane, *Soft Matter* **19**, 2654 (2023).
  - [3] M. Impérator-Clerc, P. Kalugin, S. Schenk, W. Widdra, and

- S. Förster, Higher-dimensional geometrical approach for the characterization of two-dimensional square-triangle-rhombus tilings, *Phys. Rev. B* **110**, 144106 (2024).
- [4] M. Widom, Bethe ansatz solution of the square-triangle random tiling model, *Phys. Rev. Lett.* **70**, 2094 (1993).
- [5] P. Kalugin, The square-triangle random-tiling model in the thermodynamic limit, *J. Phys. A Math. Gen.* **27**, 3599 (1994).
